# Supplementary material for: Non-Hermitian Squeezed Polarons
Source: arXiv:2202.10481 source file (2023-01-27)

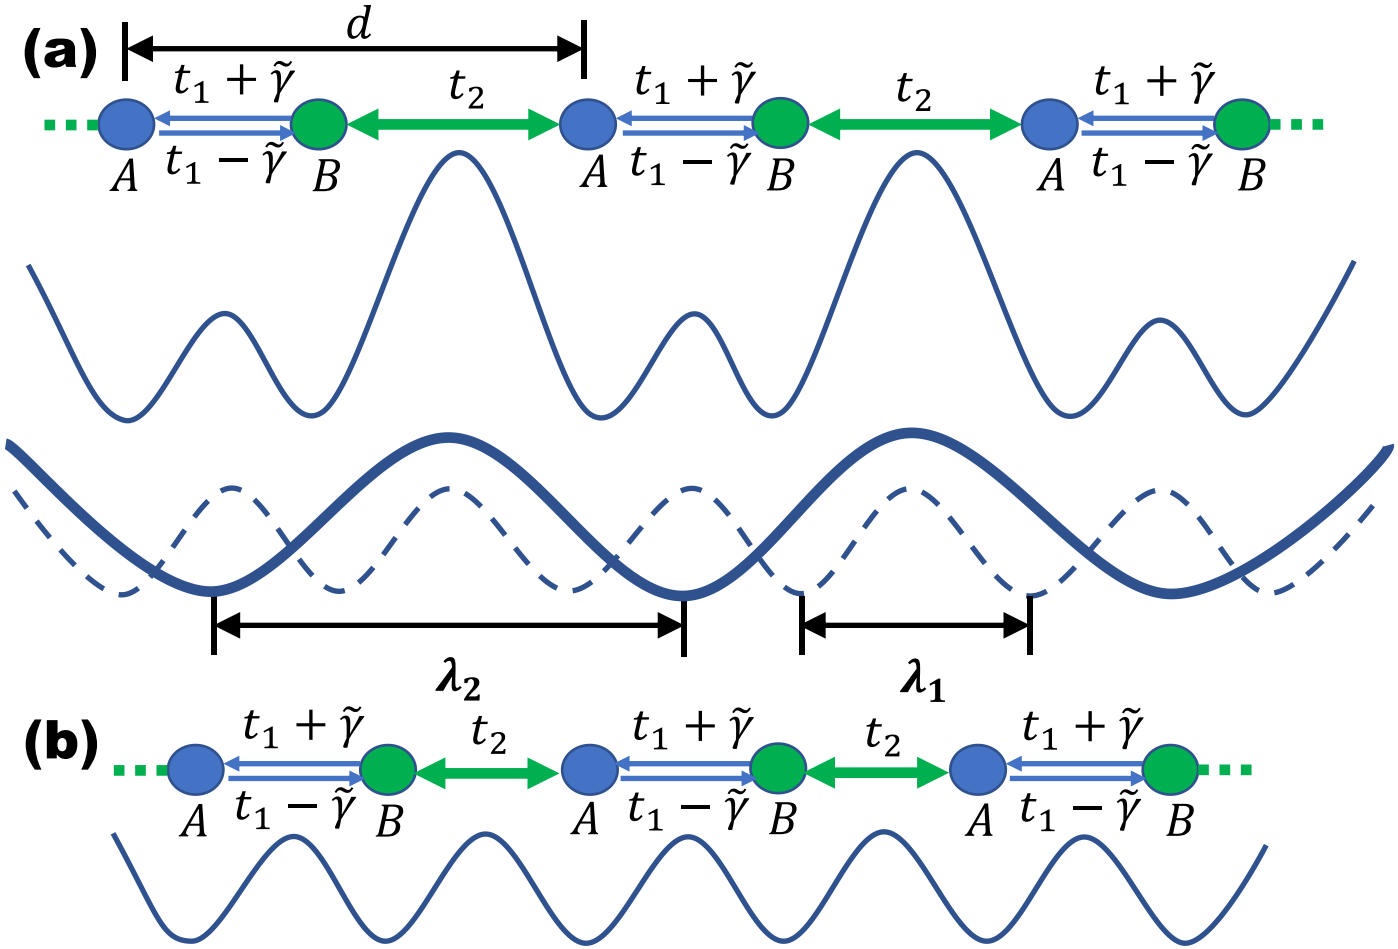

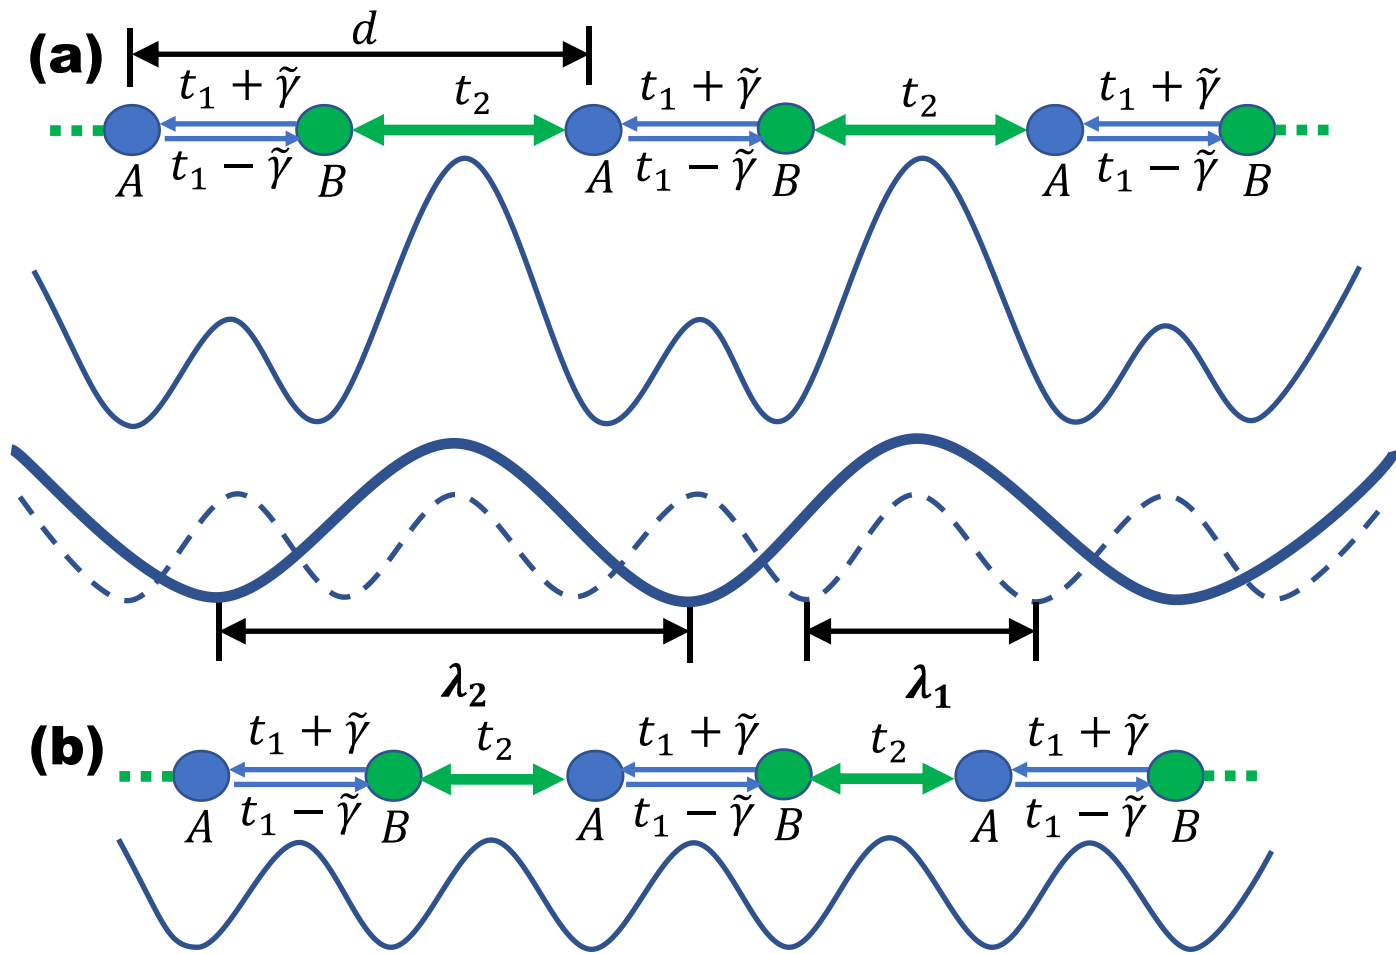

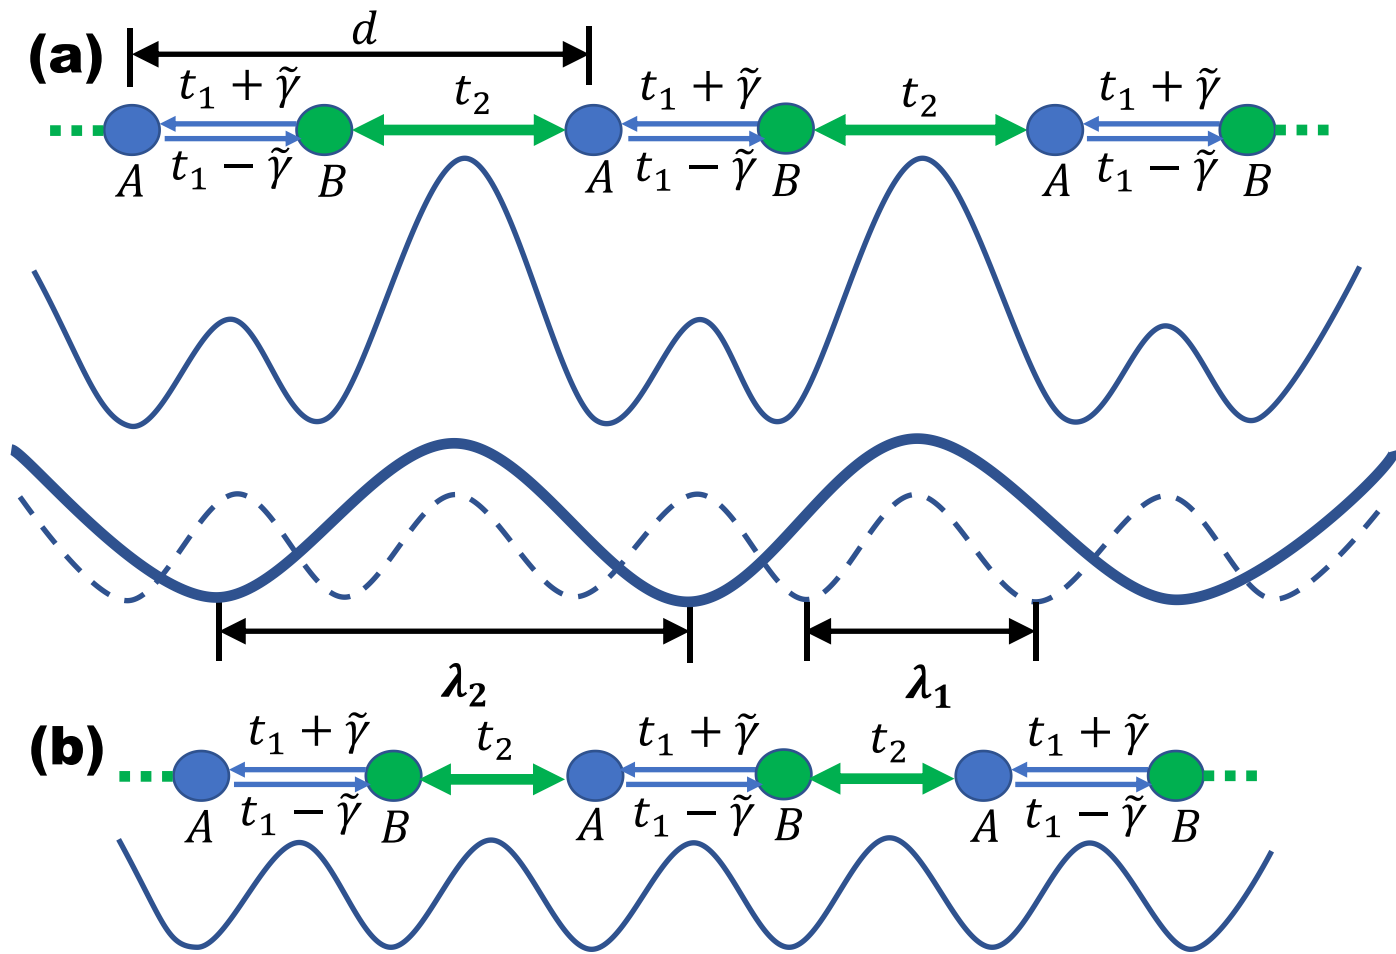

Supplement: Supplementary file 1 [file nonher-ssh-1105_supp.pdf]
